# Supplementary material for: Mechanical Search on Shelves with Efficient Stacking and Destacking of Objects
Source: arXiv:2207.02347 source file (2022-07-05)
Supplement: Supplementary file 1 [file 9-appendix.tex]

\begin{table}[h!]
    \centering
    \begin{tabular}{@{}ccccccccccccc@{}}\toprule
 Aspect   & \multicolumn{2}{c}{6 objs} & \multicolumn{2}{c}{8 objs} & \multicolumn{2}{c}{10 objs} & \multicolumn{2}{c}{12 objs} & \multicolumn{2}{c}{14 objs} & \multicolumn{2}{c}{16 objs} \\
    \cmidrule(lr){2-3} \cmidrule(lr){4-5} \cmidrule(lr){6-7} \cmidrule(lr){8-9} \cmidrule(lr){10-11} \cmidrule(lr){12-13}
 Ratio & \SR & \SA & \SR & \SA & \SR & \SA & \SR & \SA & \SR & \SA & \SR & \SA \\
% ======================= No. 6 =========================
\midrule
   1:1 & \sr{99} & \sa{2}{1}{3} & \sr{100} & \sa{3}{2}{4} & \sr{100} & \sa{4}{2}{6} & \sr{98} & \sa{4}{2}{6} & \sr{91} & \sa{4}{2}{7} & \sr{88} & \sa{4.5}{3}{7.25}\\
  
  2:1 & \sr{100} & \sa{2}{1}{3} & \sr{100} & \sa{2}{2}{4} & \sr{100} & \sa{4}{2}{5} & \sr{97} & \sa{3}{2}{6} & \sr{97} & \sa{4}{3}{8} & \sr{88} & \sa{4}{2}{7} \\
  
   4:1 & \sr{100} & \sa{2}{2}{2} & \sr{99} & \sa{2}{2}{3} & \sr{99} & \sa{3}{2}{4} & \sr{99} & \sa{3}{2}{4} & \sr{88} & \sa{3.5}{2}{6} & \sr{88} & \sa{4}{3}{6}\\
\bottomrule
    \end{tabular}
    \caption{Results of DARSS for different targets with aspect ration of 1:1, 2:1 and 4:1. }
    \label{tab:asp}
\end{table}

\begin{table}[h!]
    \centering
    \begin{tabular}{@{}ccccccccccccc@{}}\toprule
   Visibility  & \multicolumn{2}{c}{6 objs} & \multicolumn{2}{c}{8 objs} & \multicolumn{2}{c}{10 objs} & \multicolumn{2}{c}{12 objs} & \multicolumn{2}{c}{14 objs} & \multicolumn{2}{c}{16 objs} \\
    \cmidrule(lr){2-3} \cmidrule(lr){4-5} \cmidrule(lr){6-7} \cmidrule(lr){8-9} \cmidrule(lr){10-11} \cmidrule(lr){12-13}
 Threshold & \SR & \SA & \SR & \SA & \SR & \SA & \SR & \SA & \SR & \SA & \SR & \SA \\
% ======================= No. 6 =========================
\midrule
  $0.8$ & \sr{99} & \sa{2}{1}{3} & \sr{100} & \sa{3}{2}{4} & \sr{100} & \sa{4}{2}{6} & \sr{98} & \sa{4}{2}{6} & \sr{91} & \sa{4}{2}{7} & \sr{88} & \sa{4.5}{3}{7.25}\\
  
  $0.7$ & \sr{99} & \sa{2}{1}{3} & \sr{100} & \sa{3}{2}{4} & \sr{100} & \sa{4}{2}{6} & \sr{98} & \sa{4}{2}{6} & \sr{91} & \sa{4}{2}{7} & \sr{88} & \sa{4}{3}{7} \\
  
  $0.9$ & \sr{99} & \sa{2}{1}{3} & \sr{100} & \sa{3}{2}{4} & \sr{100} & \sa{4}{2}{6} & \sr{98} & \sa{4}{2}{6} & \sr{91} & \sa{4}{2}{7} & \sr{85} & \sa{5}{3}{8}\\
\bottomrule
    \end{tabular}
    \caption{Experiments results of DARSS varying visibility threshold from 0.7 to 0.9. The results difference are negligible showing the ability of the policy revealing the target reliably. }
    \label{tab:v}
\end{table}

Ablation experiments results with different target aspect ratios and different visibility threshold are shown in Table~\ref{tab:asp} and Table~\ref{tab:v}, respectively. The experiments are run over 600 scenes with 6 to 16 objects. Success rate (SR) and steps taken, shown as median (first quartile, third quartile) are reported.
